# Supplementary material for: Theory of Multiple Scattering Enhanced Single Particle Plasmonic Sensing
Source: arXiv:2105.02798 source file (2021-07-03)
Supplement: Supplementary file 1 [file Berk2021_supplement.pdf]

# Supplemental Material: Multiple Scattering Enhanced Single Particle Sensing

Joel Berk and Matthew R. Foreman\*

*Blackett Laboratory, Imperial College London, Prince Consort Road, London, United Kingdom SW7 2BW*

We are interested in the distribution, in the case of a scalar field, of  $\gamma_1 = 1 + \sum_{i=1}^N A_i$  as defined in the main text, where  $A_i = (k_0^2/\varepsilon_0) \exp[-i\mathbf{k}_{\text{out}} \cdot (\mathbf{r}_i - \mathbf{r}_{N+1})] \sum_{j=1}^N M_{ij}^{-1} \alpha G_{j,N+1}$ . We assume that the phase of  $A_i$  is uniformly distributed over the full  $2\pi$  range and independent of the amplitudes  $|A_i|$ . Making the further assumption that  $N$  is large, such that the central limit theorem can be applied, it then follows that the phasor sum  $\sum_{i=1}^N A_i$  is a zero mean complex circular Gaussian random variable with variance  $\sigma_1^2 = N\langle |A_i|^2 \rangle/2$  [1]. Consequently, the probability density function of  $\gamma_1$  is a rotationally symmetric Gaussian with mean of 1 and the same standard deviation. The amplitude  $|\gamma_1|$  in turn follows a Rician distribution. In order to calculate  $\sigma_1^2$ , we expand  $M_{ij}^{-1}$  as a Neumann series to give

$$A_i = e^{-i\mathbf{k}_{\text{out}} \cdot (\mathbf{r}_i - \mathbf{r}_{N+1})} \sum_{k=0}^{\infty} \left( \frac{k_0^2}{\varepsilon_0} \right)^{k+1} \sum_{l_1, \dots, l_{k-1}, j} \alpha G_{il_1} \alpha G_{l_1 l_2} \alpha G_{l_2 l_3} \dots \alpha G_{l_{k-2} l_{k-1}} \alpha G_{l_{k-1} j} \alpha G_{j, N+1}. \quad (1)$$

Since  $G_{l_i l_j}$  describes free propagation from  $\mathbf{r}_{l_j}$  to  $\mathbf{r}_{l_i}$  and  $\alpha$  describes a scattering event,  $A_i$  corresponds to a sum over all scattering paths visiting scatterers  $N+1 \rightarrow j \rightarrow l_{k-1} \rightarrow l_{k-2} \rightarrow \dots \rightarrow l_2 \rightarrow l_1 \rightarrow i$  and the sum implicitly excludes terms where  $l_p = l_{p+1}$  (i.e. the same scatterer is not visited consecutively). It is useful to define the sum over  $k$ , describing propagation from  $\mathbf{r}_i$  to  $\mathbf{r}$  via all scattering paths, more generally for any start and end points  $\mathbf{r}'$  and  $\mathbf{r}$  respectively. We denote this quantity  $G_{sc}(\mathbf{r}, \mathbf{r}')$  as it is (ignoring some prefactors) the Green's function for the disordered system including the  $N$  initial scatterers, and it is given by

$$G_{sc}(\mathbf{r}, \mathbf{r}') = \sum_{k=0}^{\infty} \left( \frac{k_0^2}{\varepsilon_0} \right)^{k+1} \sum_{l_1, \dots, l_k} \alpha G(\mathbf{r}, \mathbf{r}_{l_1}) \alpha G_{l_1 l_2} \alpha G_{l_2 l_3} \dots \alpha G_{l_{k-2} l_{k-1}} \alpha G_{l_{k-1} l_k} \alpha G(\mathbf{r}_{l_k}, \mathbf{r}'). \quad (2)$$

Following the approach in Ref. [2], replacing each Green's function by its Fourier decomposition and ignoring paths with repeated scatterers (i.e. assuming each  $\mathbf{r}_{l_i}$  is distinct), one can average over the intermediate scatterer positions to give

$$\begin{aligned} \langle G_{sc}(\mathbf{r}, \mathbf{r}') \rangle &= \int \left[ 1 - n\alpha \frac{k_0^2}{\varepsilon_0} \tilde{G}(\mathbf{q}) \right]^{-1} \alpha \frac{k_0^2}{\varepsilon_0} \tilde{G}(\mathbf{q}) e^{i\mathbf{q} \cdot (\boldsymbol{\rho} - \boldsymbol{\rho}')} \frac{d^2 \mathbf{q}}{(2\pi)^2} \\ &= \int \frac{-4\mu}{k_{\text{SPP}}^2 - q^2 + 4n\mu} e^{i\mathbf{q} \cdot (\boldsymbol{\rho} - \boldsymbol{\rho}')} \frac{d^2 \mathbf{q}}{(2\pi)^2}, \end{aligned} \quad (3)$$

where  $\tilde{G}(\mathbf{q}) = -4A_0 \exp(-2ak_{\text{SPP}}z_s)/[k_{\text{SPP}}^2 - q^2]$  is the transverse Fourier transform of  $G_{\text{SPP}}$  defined in Eq. (9) of the main text and  $\mu$  is also defined in the main text. Noting that averaging restores translational invariance, we can define the Fourier space representation  $\langle \tilde{G}_{sc}(\mathbf{q}) \rangle = \int \langle G_{sc}(\mathbf{r}, \mathbf{r}') \rangle \exp[-i\mathbf{q} \cdot (\boldsymbol{\rho} - \boldsymbol{\rho}')] d^2 \boldsymbol{\rho}$ , which is given by

$$\langle \tilde{G}_{sc}(\mathbf{q}) \rangle = \frac{-4\mu}{k_{\text{SPP}}^2 - q^2 + 4n\mu}. \quad (4)$$

Eq. (4) shows that the average effect of scattering is to shift the SPP wavevector [3]. In order to calculate  $\sigma_1^2$ , we must evaluate  $\langle A_i A_i^* \rangle = \langle G_{sc}(\mathbf{r}_i, \mathbf{r}_{N+1}) G_{sc}^*(\mathbf{r}_i, \mathbf{r}_{N+1}) \rangle$ . As  $G_{sc}$  is a sum over all multiple scattering paths,  $|A_i|^2$  contains the interference of all paths. Within the ladder approximation, we assume that the phase difference between different scattering paths mean they will tend to average out over realisations unless they are identical (i.e. visit the same scatterers in the same order) [4]. This allows  $\langle |A_i|^2 \rangle$  to be expressed as

$$\begin{aligned} \langle |A_i|^2 \rangle &= \int \langle G_{sc}(\mathbf{r}_i, \mathbf{r}_{N+1}) \rangle \langle G_{sc}^*(\mathbf{r}_i, \mathbf{r}_{N+1}) \rangle \frac{d^2 \boldsymbol{\rho}_i}{L^2} \\ &+ \sum_{k=1}^{\infty} \sum_{s_1, \dots, s_k=1}^N \int |\langle G_{sc}(\mathbf{r}_i, \mathbf{r}_{s_1}) \rangle \langle G_{sc}(\mathbf{r}_{s_1}, \mathbf{r}_{s_2}) \rangle \langle G_{sc}(\mathbf{r}_{s_2}, \mathbf{r}_{s_3}) \rangle \dots \langle G_{sc}(\mathbf{r}_{s_k}, \mathbf{r}_{N+1}) \rangle|^2 \frac{d^2 \boldsymbol{\rho}_i}{L^2} \frac{d^2 \boldsymbol{\rho}_{s_1}}{L^2} \frac{d^2 \boldsymbol{\rho}_{s_2}}{L^2} \dots \frac{d^2 \boldsymbol{\rho}_{s_k}}{L^2}, \end{aligned} \quad (5)$$

where the first term is the contribution from the interference of paths sharing no scatterers and each term in the sum over  $k$  is the contribution from the interference between one path from  $A_i$  visiting  $k$  scatterers  $s_1, s_2, \dots, s_k$  and a conjugated path (from  $A_i^*$ ) visiting the same  $k$  scatterers in the same order. In using  $\langle G_{sc} \rangle$  instead of  $G_{\text{SPP}}$  to propagate between each of these  $k$  shared scatterers, we account for any scattering during this propagation from other scatterers outside this set of  $k$  scatterers. The integration  $\int \dots d^2 \rho_{s_j} / L^2$  arises from averaging over the scatterer positions. Inserting the Fourier decomposition  $\langle G_{sc}(\mathbf{r}, \mathbf{r}') \rangle = \int \langle \tilde{G}_{sc}(\mathbf{q}) \rangle \exp[i\mathbf{q} \cdot (\boldsymbol{\rho} - \boldsymbol{\rho}')] d^2 \mathbf{q} / (2\pi)^2$  for each factor of  $\langle G_{sc} \rangle$  results in

$$\begin{aligned} \langle |A_i|^2 \rangle &= \frac{1}{L^2} \int \left| \langle \tilde{G}_{sc}(\mathbf{q}) \rangle \right|^2 d^2 \mathbf{q} / (2\pi)^2 \\ &+ \sum_{k=1}^{\infty} \sum_{s_1, \dots, s_k=1}^N \int \langle \tilde{G}_{sc}(\mathbf{q}_1) \rangle \langle \tilde{G}_{sc}(\mathbf{q}_2) \rangle \dots \langle \tilde{G}_{sc}(\mathbf{q}_k) \rangle \langle \tilde{G}_{sc}^*(\mathbf{q}'_1) \rangle \langle \tilde{G}_{sc}^*(\mathbf{q}'_2) \rangle \dots \langle \tilde{G}_{sc}^*(\mathbf{q}'_k) \rangle \\ &\times e^{i(\mathbf{q}_1 - \mathbf{q}'_1) \cdot (\boldsymbol{\rho}_i - \boldsymbol{\rho}_{s_1})} e^{i(\mathbf{q}_2 - \mathbf{q}'_2) \cdot (\boldsymbol{\rho}_{s_1} - \boldsymbol{\rho}_{s_2})} \dots e^{i(\mathbf{q}_k - \mathbf{q}'_k) \cdot (\boldsymbol{\rho}_{s_k} - \boldsymbol{\rho}_{N+1})} \frac{d^2 \boldsymbol{\rho}_i}{L^2} \frac{d^2 \boldsymbol{\rho}_{s_1}}{L^2} \frac{d^2 \boldsymbol{\rho}_{s_2}}{L^2} \dots \frac{d^2 \boldsymbol{\rho}_{s_k}}{L^2} \\ &\times \frac{d^2 \mathbf{q}_1}{(2\pi)^2} \frac{d^2 \mathbf{q}'_1}{(2\pi)^2} \frac{d^2 \mathbf{q}_2}{(2\pi)^2} \frac{d^2 \mathbf{q}'_2}{(2\pi)^2} \dots \frac{d^2 \mathbf{q}_k}{(2\pi)^2} \frac{d^2 \mathbf{q}'_k}{(2\pi)^2}. \end{aligned} \quad (6)$$

Integrating over each position gives a factor  $(2\pi)^2 \delta(\mathbf{q}_i - \mathbf{q}'_i) / L^2$ , while the sum over scatterers  $\sum_{s_1, \dots, s_k}$  reduces to a factor of  $N^k$ . Therefore, Eq. (6) becomes

$$\langle |A_i|^2 \rangle = \frac{1}{L^2} \int \left| \langle \tilde{G}_{sc}(\mathbf{q}) \rangle \right|^2 d^2 \mathbf{q} / (2\pi)^2 + \sum_{k=1}^{\infty} N^k \left( \frac{1}{L^2} \int \left| \langle \tilde{G}_{sc}(\mathbf{q}) \rangle \right|^2 \frac{d^2 \mathbf{q}}{(2\pi)^2} \right)^{k+1}. \quad (7)$$

The integral can be evaluated, resulting in

$$\begin{aligned} \int \left| \langle \tilde{G}_{sc}(\mathbf{q}) \rangle \right|^2 \frac{d^2 \mathbf{q}}{(2\pi)^2} &= \int \frac{16|\mu|^2}{(k_{\text{SPP}}^2 - q^2 + 4n\mu)(k_{\text{SPP}}^{*2} - q^2 + 4n\mu^*)} \frac{d^2 \mathbf{q}}{(2\pi)^2} \\ &= \frac{4|\mu|^2}{\text{Im}[k_{\text{SPP}}^2 + 4n\mu]} \\ &= \frac{\sigma_{\text{SPP}}}{l_{\text{abs}}^{-1} + 4n \text{Im}[\mu] / \text{Re}[k_{\text{SPP}}]}. \end{aligned} \quad (8)$$

Therefore, Eq. (7) reduces to

$$\langle |A_i|^2 \rangle = \frac{1}{L^2} \frac{\sigma_{\text{SPP}}}{l_{\text{abs}}^{-1} + 4n \text{Im}[\mu] / \text{Re}[k_{\text{SPP}}]} + \frac{1}{L^2} \sum_{k=1}^{\infty} \left( \frac{N}{L^2} \right)^k \left( \frac{\sigma_{\text{SPP}}}{l_{\text{abs}}^{-1} + 4n \text{Im}[\mu] / \text{Re}[k_{\text{SPP}}]} \right)^{k+1}. \quad (9)$$

Using  $\sigma_1^2 = N \langle |A_i|^2 \rangle / 2$ , recalling  $n = N / L^2$  and  $n\sigma_{\text{SPP}} = l_s^{-1}$  gives

$$\begin{aligned} \sigma_1^2 &= \frac{1}{2} \sum_{k=1}^{\infty} \left( \frac{l_s^{-1}}{l_{\text{abs}}^{-1} + 4n \text{Im}[\mu] / \text{Re}[k_{\text{SPP}}]} \right)^k \\ &= \frac{1}{2} \frac{l_s^{-1}}{l_{\text{abs}}^{-1} + 4n \text{Im}[\mu] / \text{Re}[k_{\text{SPP}}] - l_s^{-1}} \end{aligned} \quad (10)$$

which is the result in Eq. (10) in the main text.

---

\* matthew.foreman@imperial.ac.uk

- [1] J. Goodman, *Speckle Phenomena in Optics: Theory and Applications* (Roberts & Company, 2007).
- [2] J. Berk and M. R. Foreman, “Role of Multiple Scattering in Single Particle Perturbations in Absorbing Random Media,” submitted (2021).
- [3] A. Maradudin and W. Zierau, “Effects of surface roughness on the surface-polariton dispersion relation,” *Phys. Rev. B* **14**, 484–499 (1976).
- [4] E. Akkermans and G. Montambaux, *Mesoscopic Physics of Electrons and Photons* (Cambridge University Press, 2007), 1st ed.
